# Supplementary material for: VoronoiPatches: Evaluating A New Data Augmentation Method
Source: arXiv:2212.10054 source file (2022-12-23)
Supplement: Supplementary file 1 [file 8_appendix.tex]

\section*{\uppercase{Appendix}}

If any, the appendix should appear directly after the
references without numbering, and not on a new page. To do so please use the following command:
\textit{$\backslash$section*\{APPENDIX\}}
